# Supplementary material for: Apprentice for Event Generator Tuning
Source: arXiv:2103.05748 source file (2021-03-09)

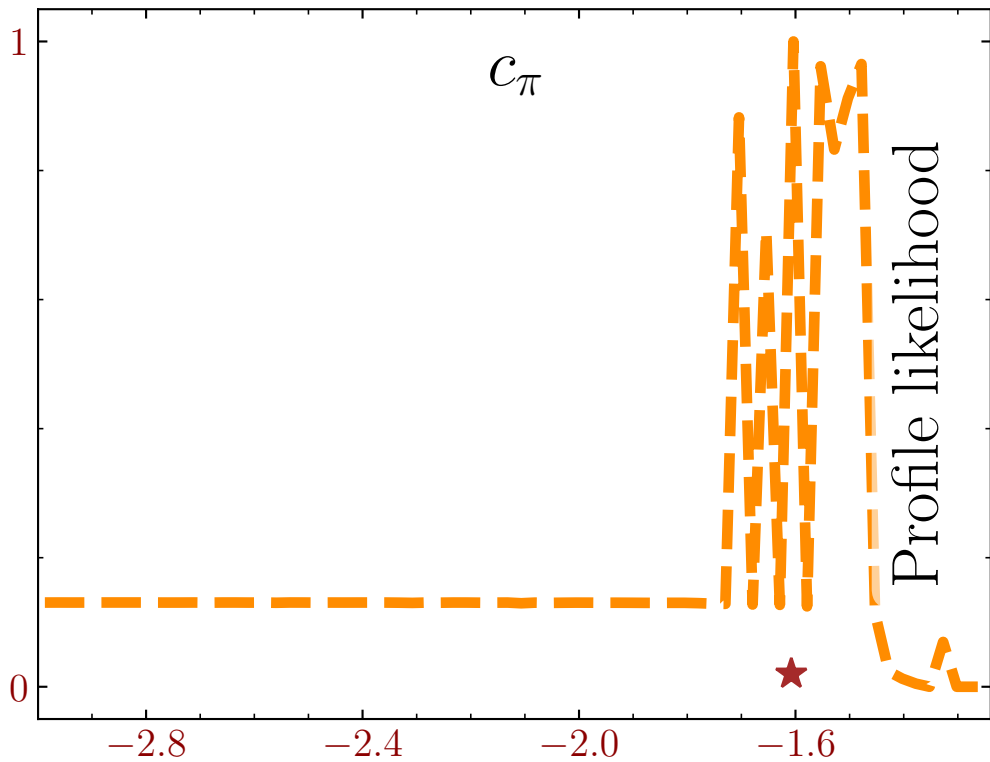





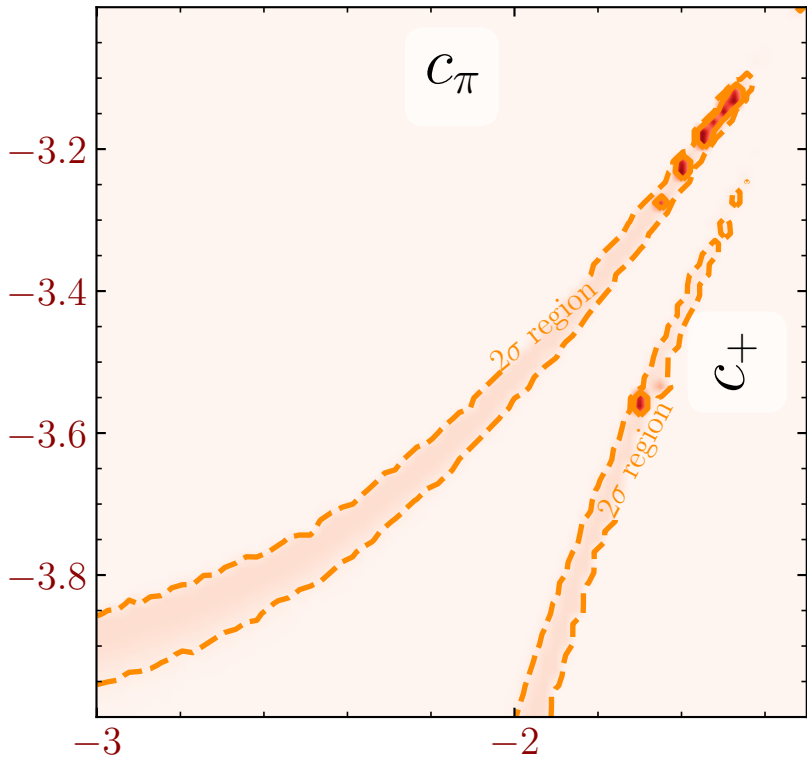

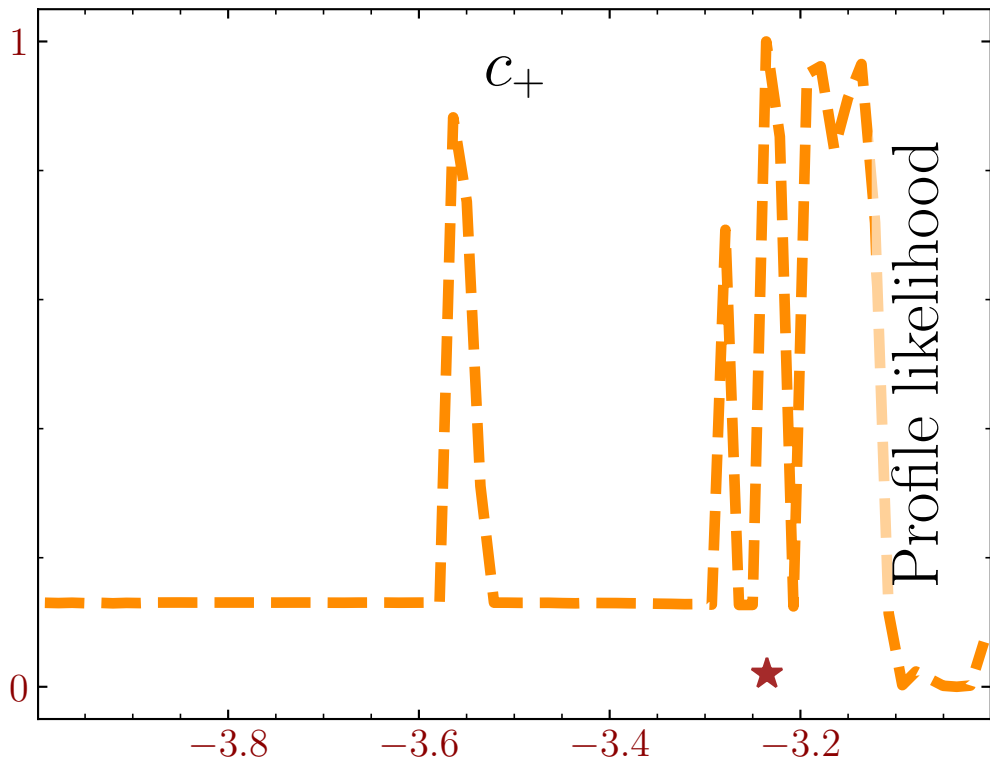



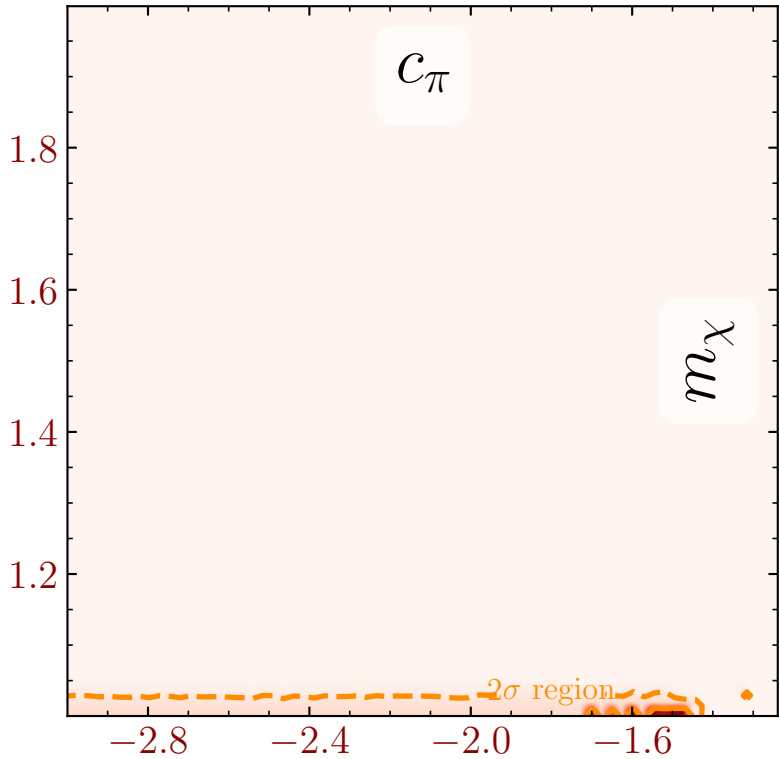

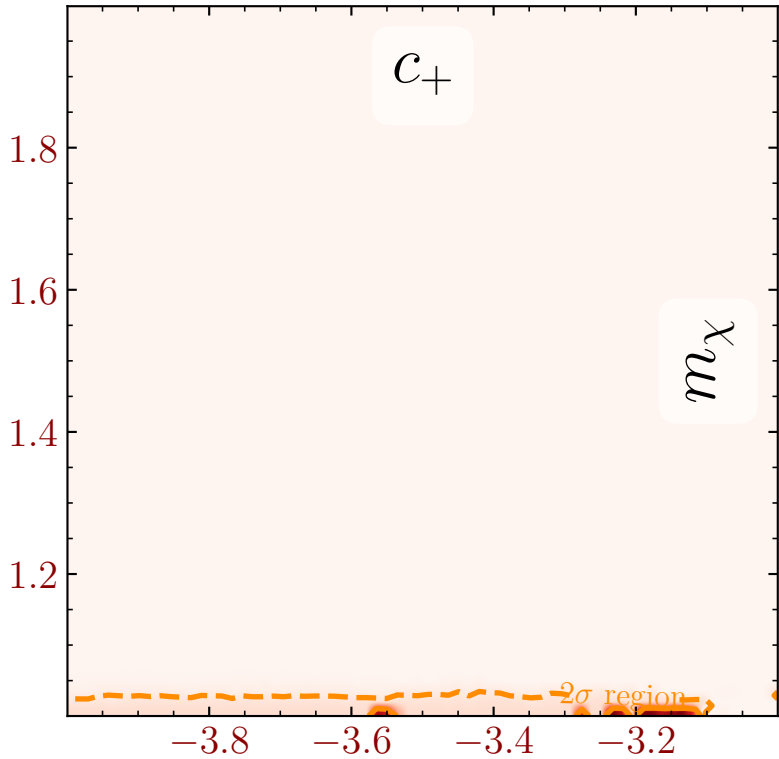

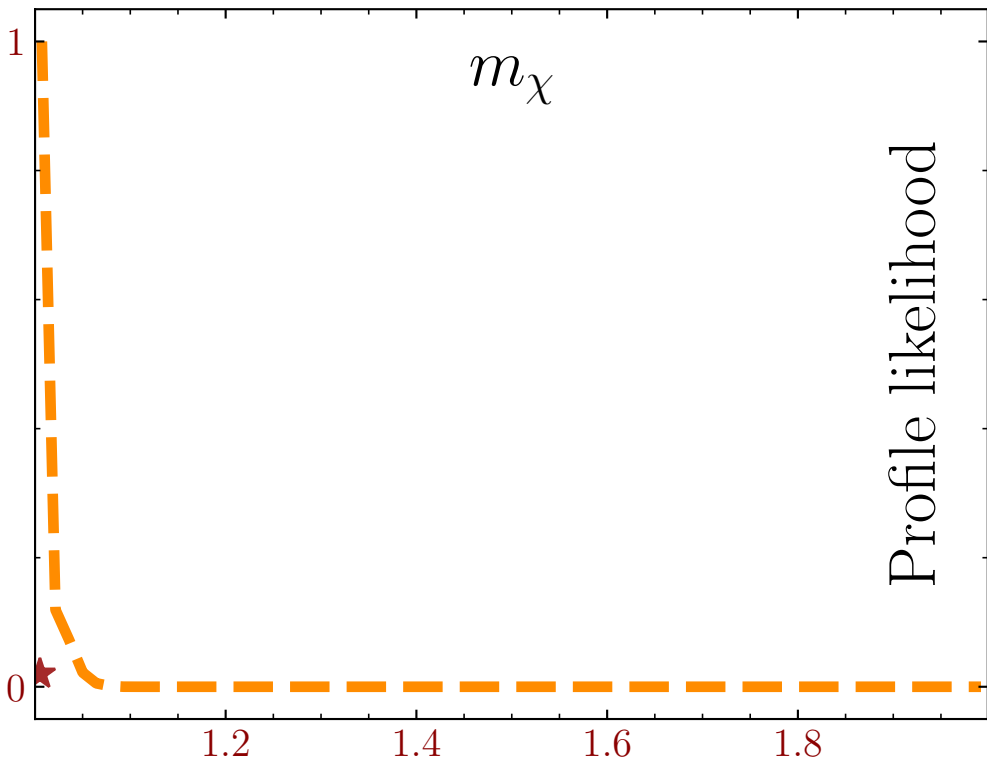

Supplement: Supplementary file 1 [file triangle2.pdf]
