# Supplementary material for: Apprentice for Event Generator Tuning
Source: arXiv:2103.05748 source file (2021-03-09)

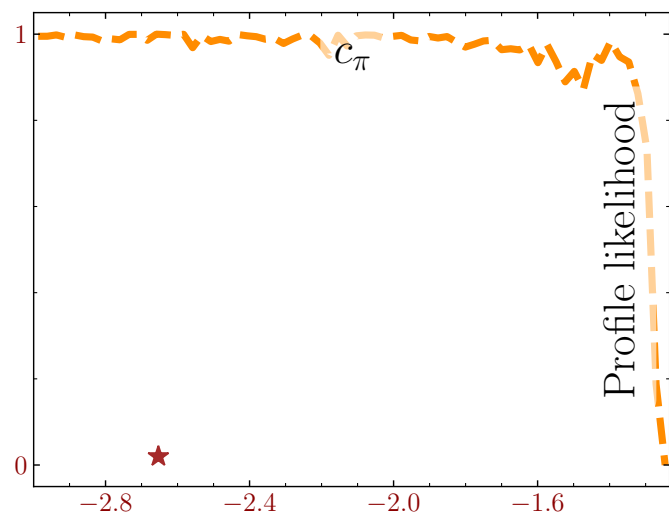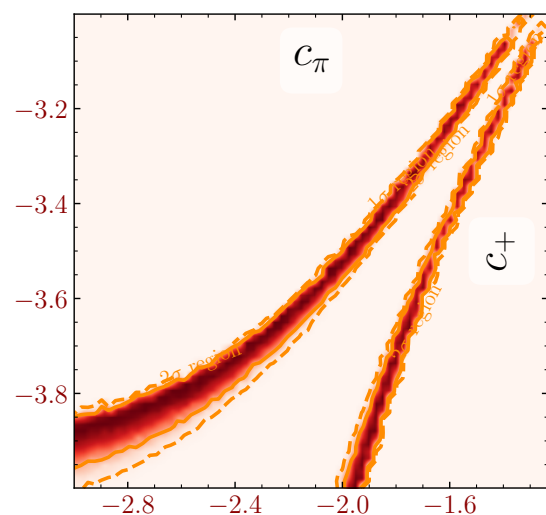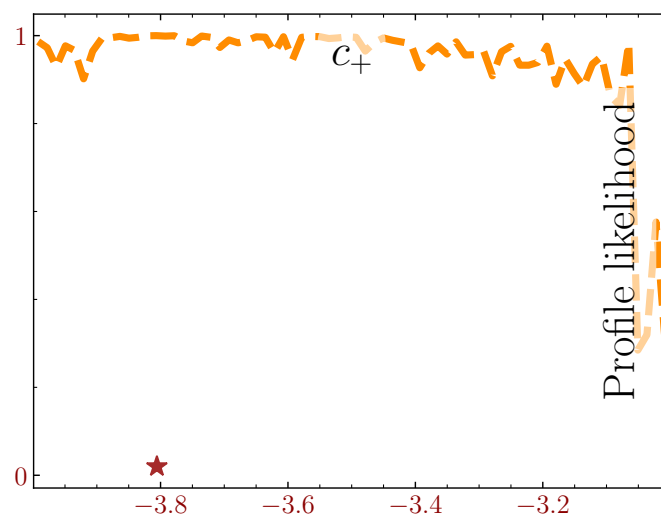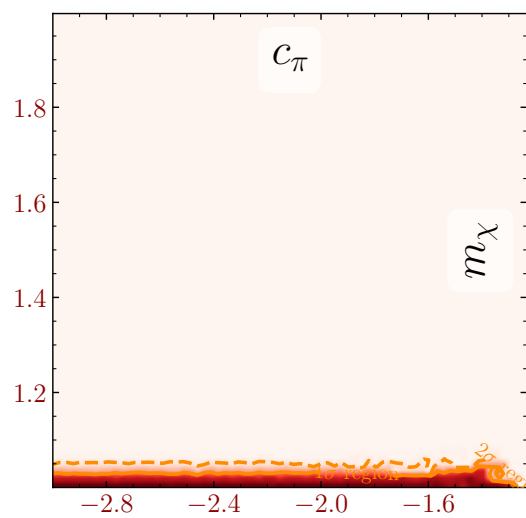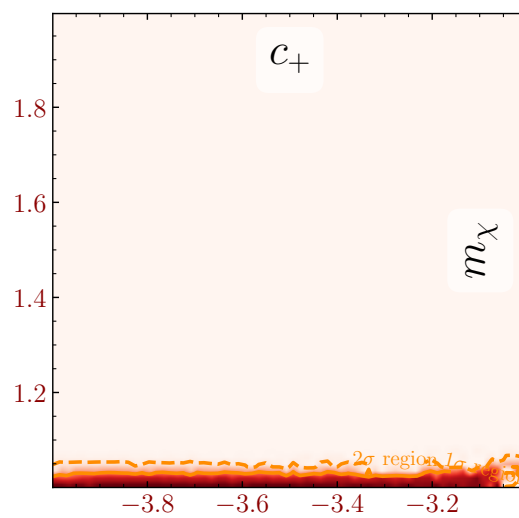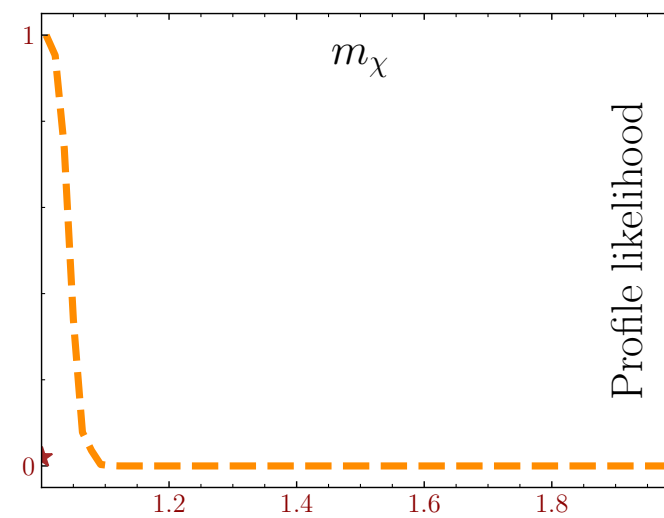

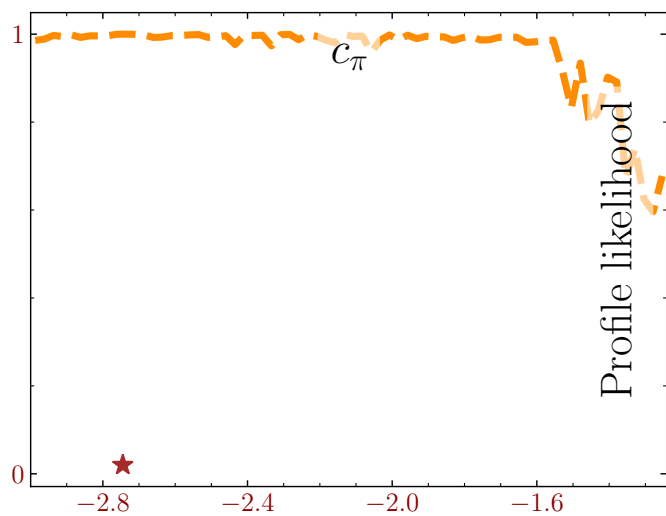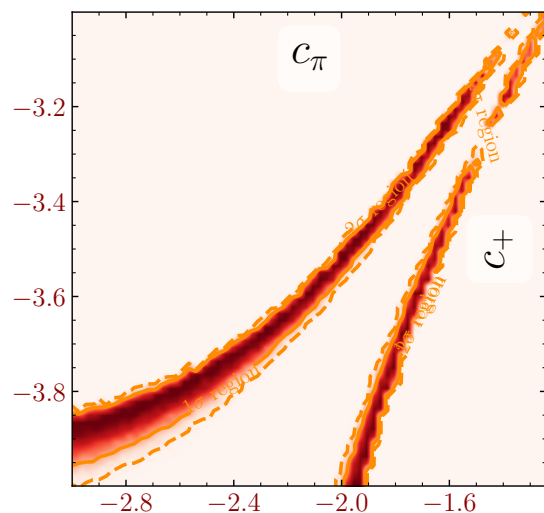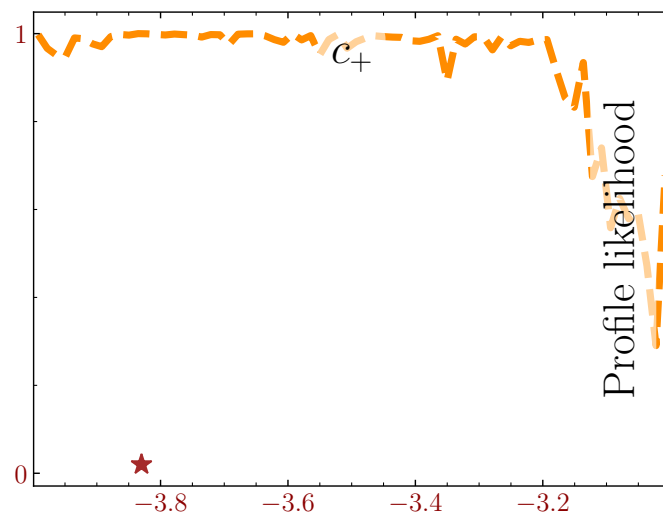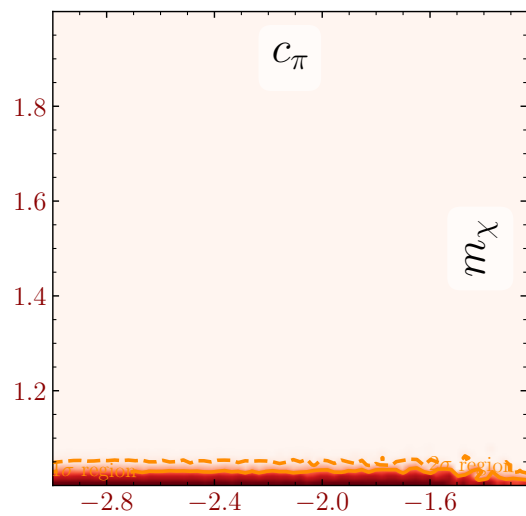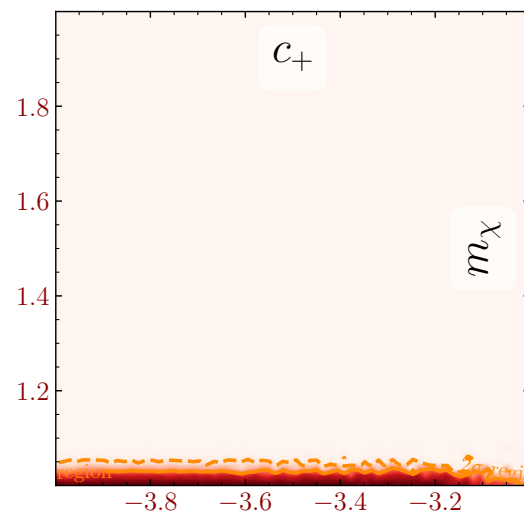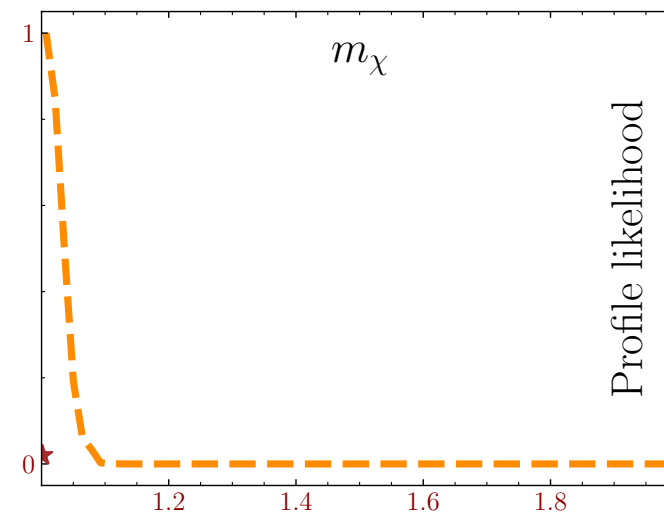

Supplement: Supplementary file 2 [file cmp.pdf]
