# Supplementary material for: Apprentice for Event Generator Tuning
Source: arXiv:2103.05748 source file (2021-03-09)

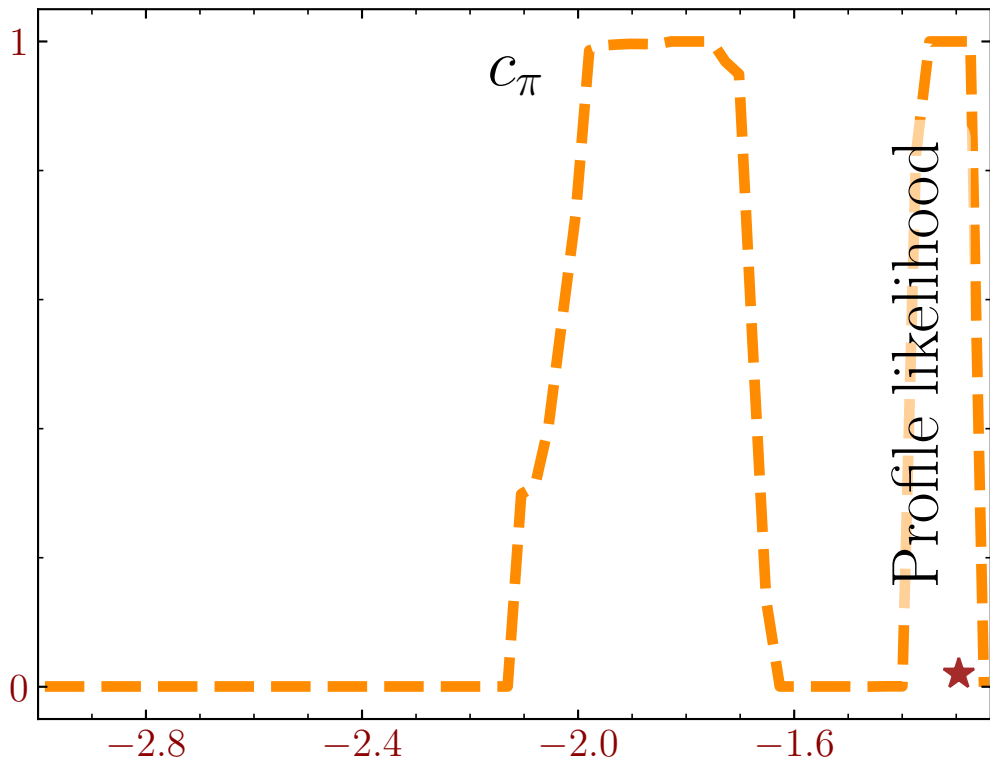





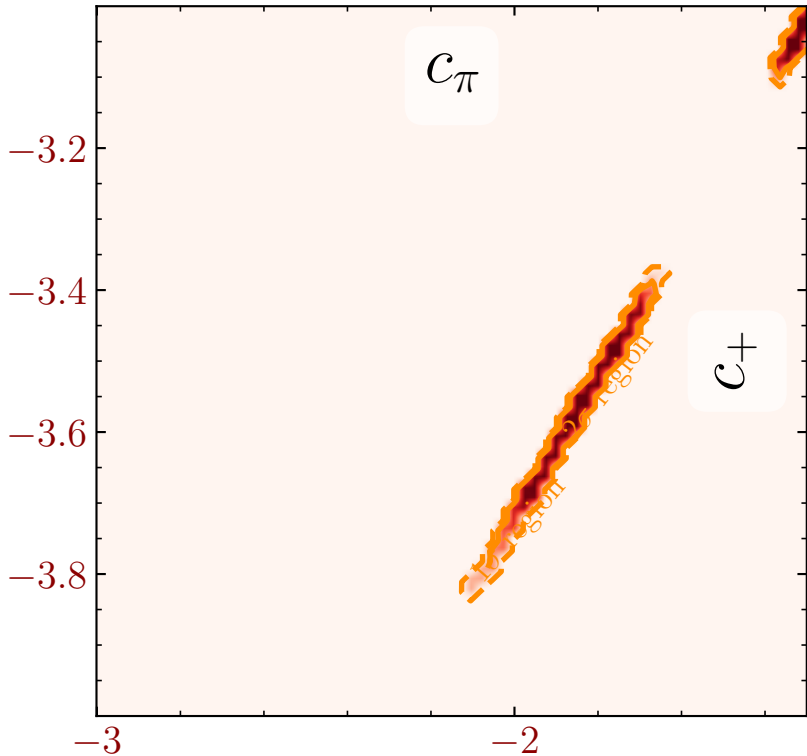

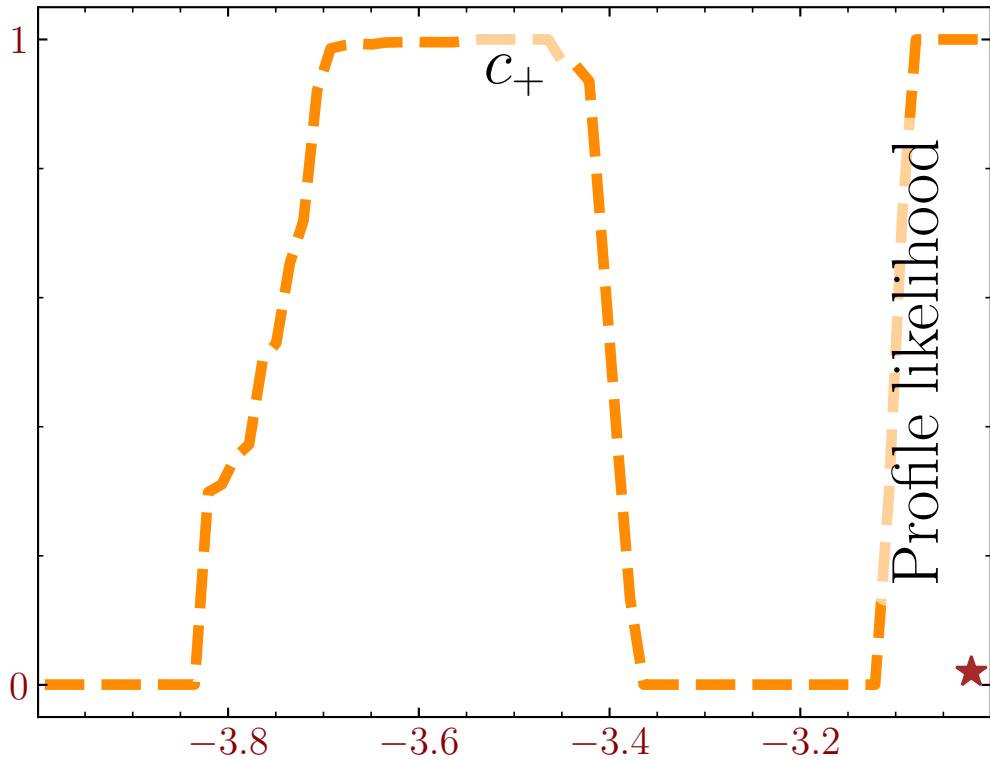



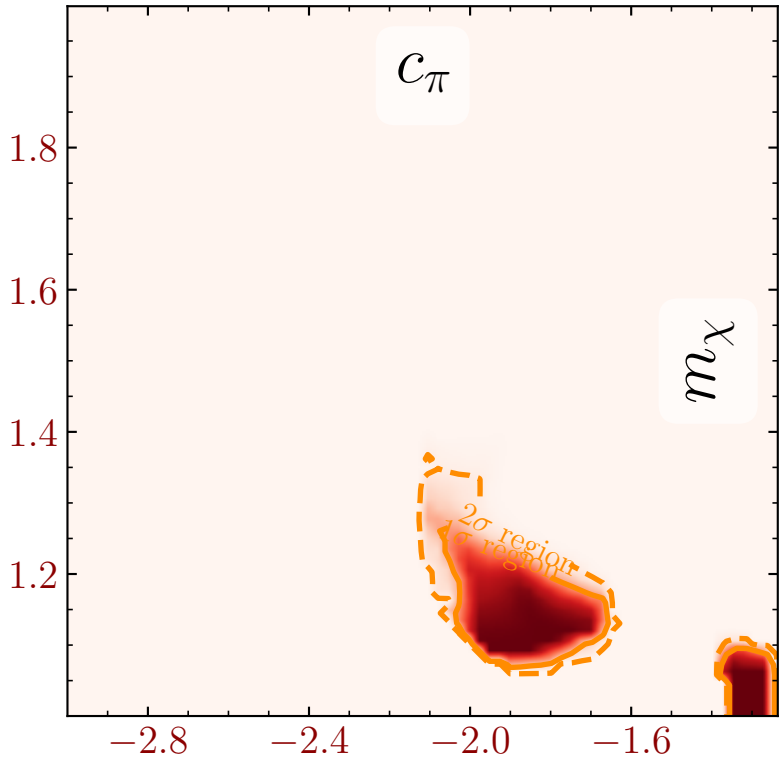

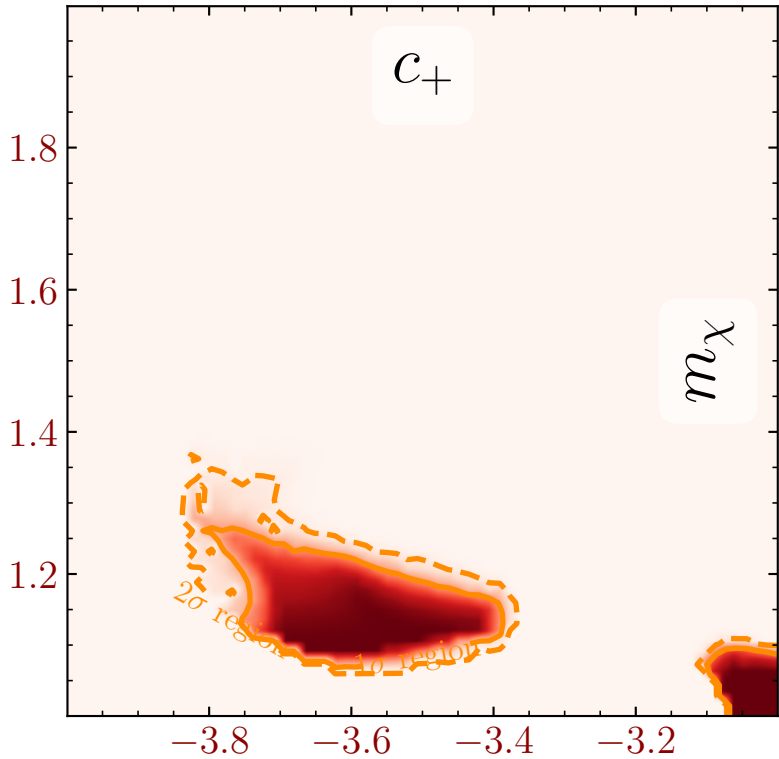



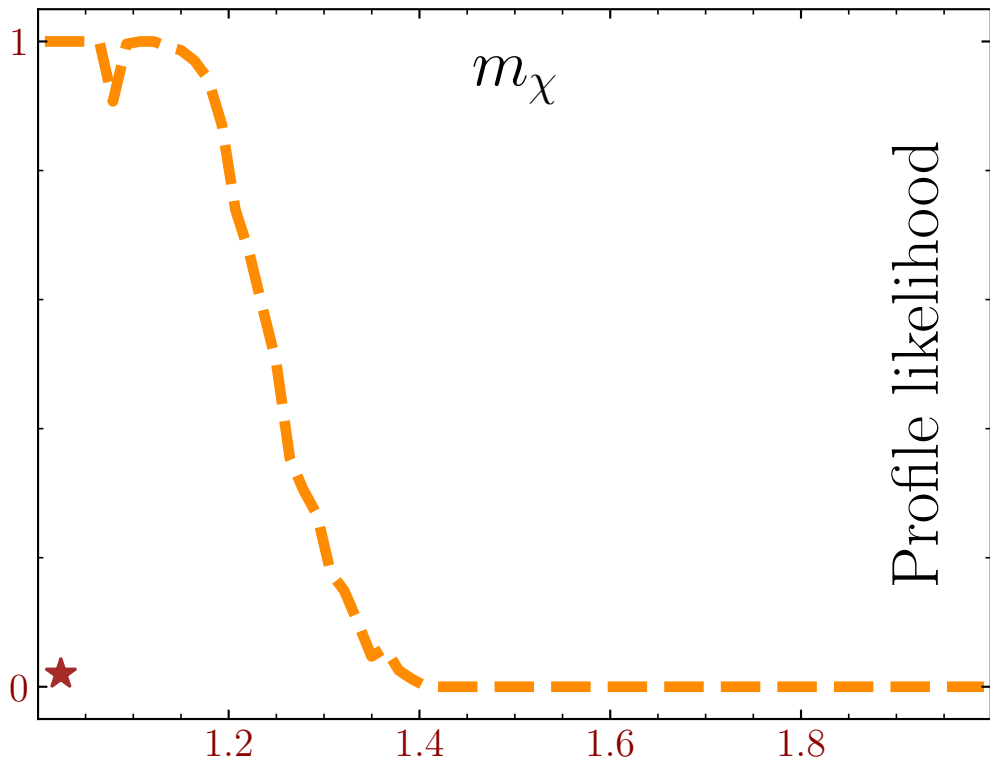

Supplement: Supplementary file 5 [file triangle2.pdf]
